# Supplementary material for: Design-Time Quantification of Integrity in Cyber-Physical-Systems
Source: arXiv:1708.04798 source file (2017-08-16)
Supplement: Supplementary file 1 [file appendix.tex]

%!TEX root = ../EGRM-ESORICS-LNCS.tex

% do not use \section anymore after \appendix, only \section*
% is possibly needed

\section*{Appendix}
\textbf{Attacker 3} controls the $in$ valve, so she can set any value for $\hat{u}_{in}(k)$ at any time $k$. Consider the $\High$-equivalent abstract states
\begin{align}
cps(0)&=((L,\rho gL),\AsSequence{open,close},\AsSequence{0,0}, L)\\
cps'(0)&=((L,\rho gL),\AsSequence{close,close},\AsSequence{0,0}, L);
\end{align}
according to the semantics $\TheSystem$ of the CPS, we have (changes underlined)
\begin{align}
cps(1)&=((L,\rho gL),\AsSequence{open,close},\AsSequence{\underline{1},0},L)\\
cps'(1)&=((L,\rho gL),\AsSequence{close,close},\AsSequence{0,0}, L)\\
cps(2)&=((L,\rho gL),\AsSequence{open,close},\AsSequence{1,0}, {\underline{L+Q_{in}}})\\
cps'(2)&=((L,\rho gL),\AsSequence{close,close},\AsSequence{0,0},{L});
\end{align}
States $cps(2)$ and $cps'(2)$ are not $\hat{y}$-equivalent, so the system does not satisfy noninterference. 

\textbf{Attacker 4} controls the water level sensor, so she can set any value for ${y}_{l}(k)$ at any time $k$. Now, consider the $\High$-equivalent abstract states
\begin{align}
cps(0)&=((L^-,\rho gL),\AsSequence{close, close},\AsSequence{0,0}, L)\\
cps'(0)&=((L^+,\rho gL),\AsSequence{close,close},\AsSequence{0,0}, L);
\end{align}
according to the semantics $\TheSystem$ of the CPS, we have (changes underlined)
\begin{align}
cps(1)&=((L^-,\rho gL),{\AsSequence{\underline{open}, close}},\AsSequence{{0},{0}}, L)\\
cps'(1)&=((L^+,\rho gL),\AsSequence{close,\underline{open}},\AsSequence{0,{0}}, L)\\
cps(2)&=((L^-,\rho gL),{\AsSequence{open, close}},\AsSequence{\underline{1},0}, L)\\
cps'(2)&=((L^+,\rho gL),\AsSequence{close,open},\AsSequence{0,\underline{1}}, L)\\
cps(3)&=((L^-,\rho gL),\AsSequence{open,close},\AsSequence{1,0}, {\underline{L+Q_{in}}})\\
cps'(3)&=((L^+,\rho gL),\AsSequence{close, open},\AsSequence{0,1}, \underline{L-Q_{out}});
\end{align}
States $cps(3)$ and $cps'(3)$ are not $\hat{y}$-equivalent, so the system does not satisfy noninterference.
